# Supplementary material for: First Dark Matter Constraints from a SuperCDMS Single-Charge Sensitive Detector
Source: arXiv:1804.10697 ancillary file (2020-12-23)
Supplement: Supplementary file 1 [file HVeV_Run_1_Data_Release.pdf]

# HVeV Run 1 Data Release

SuperCDMS Collaboration

April 1, 2019

This document accompanies the public release of data from the first run (Run1) of the SuperCDMS quantization-sensitive detector (HVeV). The dark matter (DM) search results from these data are found in <https://arxiv.org/abs/1804.10697> [1]. All experimental data required for DM searches are included in the release. The limit setting technique used in Ref [1] is also described. The provided data and information allows the community to use these data for their own analyses or for reproducing the HVeV Run 1 results. Questions about this release should be directed to [supercdms\\_publications@lists.astro.caltech.edu](mailto:supercdms_publications@lists.astro.caltech.edu).

The provided experimental and supplemental data files and information are described in Sec. 1. Due to the discrete nature of any expected signal in the HVeV detector the signal expectation has to be converted from a continuous spectrum in deposited energy into a discrete spectrum in produced electron-hole pairs ( $e^-h^+$ ). This conversion requires an ionization model that depends on the Fano factor  $F$  and is described in Sec. 2. The probed DM models and the conversion of the final spectrum into the physics limits are described in Sec. 3. The published upper limits on dark photon absorption and light DM-electron scattering were computed using the high-statistics Optimum Interval (OI) method [2]. The background was assumed to be completely unknown for this analysis in order to set a conservative limit.

## 1 Description of the Files

Eight tab separated value files (.tsv) are included in this data release and can be found in the different directories of the accompanying .zip file. The names and descriptions of these files are provided in this section.

### 1.1 HVeV data

The released HVeV data files are listed and described in this section. The two respective files contain the signal efficiency and the observed spectrum after all selection cuts have been applied. The data that were used for the HVeV results are included in the files. In the case of the efficiency file, two additional efficiency curves are included, which allow the user to apply a different analysis approach than chosen for Ref [1] and to explore impacts on the computed limit. Using an alternative efficiency curve should only improve the limit, given our conservative analysis approach in Ref [1].

#### 1.1.1 Energy Spectrum: `eventEnergy_ehpairs_Neg140.tsv`

The final energy spectrum used for the HVeV DM search results is shown in Fig. 1 in units of  $e^-h^+$  pairs. All events contributing to this spectrum are listed in `eventEnergy_ehpairs_Neg140.tsv` and sorted by increasing energy. These are only events that survived all analysis cuts. The spectrum shown in Fig. 1 can be reproduced by choosing a bin width of  $0.02 e^-h^+$  pairs. For this analysis, only data up to  $10 e^-h^+$  pairs were included in the limit calculations, but data above this cut-off are included in this data release.

#### 1.1.2 Efficiency: `efficiency_ehpairs_Neg140_all.tsv`

Figure 2a shows the signal efficiency after quality cuts were applied, including the poisson uncertainty due to the number of events in each bin. It also shows the best fit of a sigmoid efficiency model after all cuts were applied.

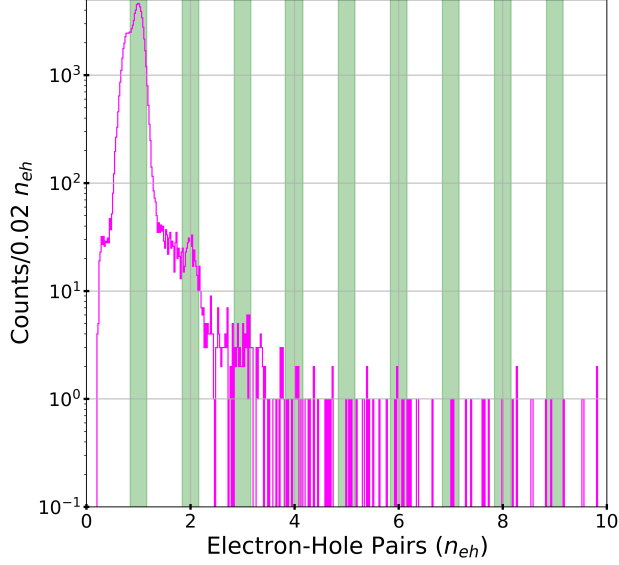

Figure 1: HVeV Run 1 DM search data after all selection cuts are applied (pink). The green shaded bands mark the ROI for the DM searches in [1], i.e. the  $\pm 2\sigma_{eh}$  regions for each quantization peak with  $\sigma_{eh} = 0.09$   $e^-h^+$  pairs.

In the analysis carried out for Ref [1], the region of interest (ROI) is exclusively within  $\pm 2\sigma_{eh}$  of the quantization peaks, the DM signal region. In order to obtain this ROI, the efficiency is set to zero outside this region. The resulting efficiency curve for this method is shown in Fig. 2b. Finally, the large uncertainty in the efficiency at high energies was accounted for by a fit to the lower error bounds in Fig. 2a resulting in the conservative efficiency curve shown in Fig. 2c. This last curve was used for the final results.

All three efficiency curves are included in `efficiency_ehpairs_Neg140_all.tsv` with the following structure:

- Column 0: energy in  $e^-h^+$  pairs.
- Column 1: best fit efficiency model (Fig. 2a).
- Column 2: best fit efficiency model with regions outside  $\pm 2\sigma_{eh}$  of the peaks set to zero (Fig. 2b). Using this efficiency effectively selects the in-peaks ROI.
- Column 3: conservative efficiency model (fit to lower error bound) with regions outside  $\pm 2\sigma_{eh}$  of the peaks set to zero (Fig. 2c).

For the limit calculation, Column 3 was used.

## 1.2 Supplementary Data: Complex Conductivity

The files in this section do not contain SuperCDMS data. They contain external complex conductivity,  $\tilde{\sigma}$ , data that is necessary to calculate the published dark photon kinetic mixing limit (see also Sec. 3.2.2). The real and imaginary parts in  $\tilde{\sigma} = \sigma_1 + i\sigma_2$  are included in separate files and are also described separately in this section.

### 1.2.1 Real Part of the Complex Conductivity: Photoelectric Cross Section

The photoelectric cross section corresponds to the real part of the complex conductivity,  $\sigma_1$ . The  $\sigma_1$  information is typically provided either in units of an absorption coefficient ( $\text{cm}^2/\text{g}$ ) or in units of the conductivity (eV). The notation in Ref [1], and in Eq. 16, requires the conductivity scale and was used to calculate the official results. The photon energy scale on the x-axis is in keV. The x- and y-axis scales are referred to in the file names (`photoelectric.absorption...<x-axis scale>_<y-axis scale>.tsv`):

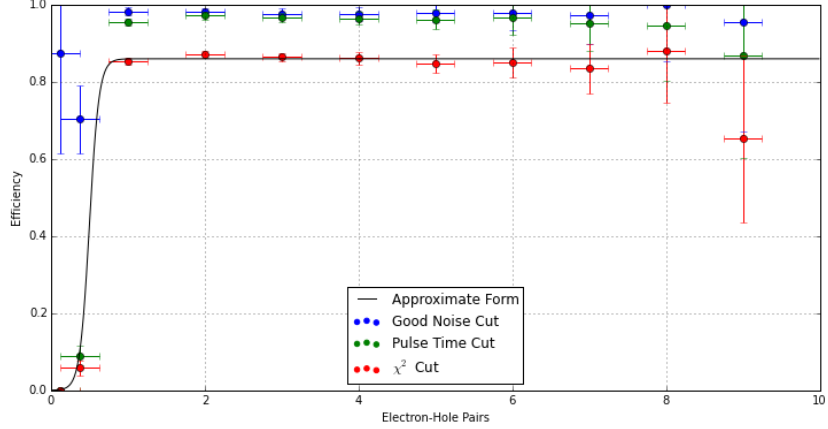

(a) Efficiency of livetime, pulse trigger time, and chi-square cuts as a function of number of  $e^-h^+$  pair number as determined from the laser calibration data (each cut includes the previous cuts as well). A sigmoid function is fit to the cumulative cut efficiency, shown as a solid line.

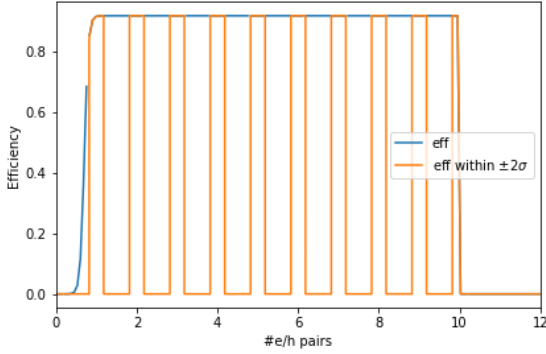

(b) Best fit efficiency (blue) with regions outside  $\pm 2\sigma_{eh}$  of the peaks set to zero (orange).

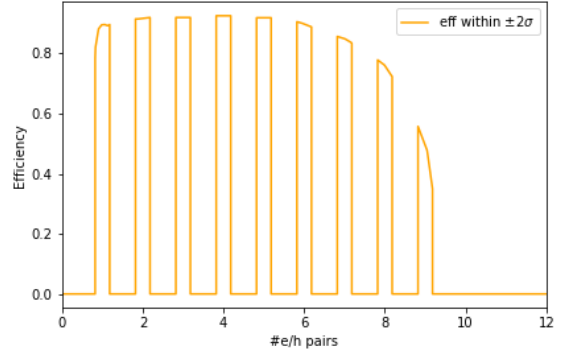

(c) Conservative efficiency after fitting to the lower error bounds in Fig. 2a. The regions outside  $\pm 2\sigma_{eh}$  of the peaks are set to zero.

Figure 2: Event selection efficiency. The efficiency shown in (c) was used for the official results. The width of each band in (b) and (c) is defined by the resolution  $\sigma_{eh} = 0.09 e^-h^+$  pairs.

- photoelectric\_absorption\_Si\_ConservativeEnvelope\_keV\_eV.tsv,
- photoelectric\_absorption\_Si\_ReferenceData\_keV\_eV.tsv

Two versions of  $\sigma_1$  are included in the data release. One is referred to as “reference data”, which is the  $\sigma_1$  that is commonly used in dark photon absorption searches by other collaborations and scientists (as e.g. in Hochberg et al. [3]). The other one is referred to as “conservative envelope”, which represents the lowest reasonable cross section taking measurement uncertainties, temperature effects, and electric field effects into account. Those effects were studied in detail in the ancillary file of Ref [1]. They are pronounced near the indirect and the direct band gap and thus well within the energy region accessible by the HVeV detector. The nominal dark photon kinetic mixing limit was calculated with the “reference data” and a band was added to the limit using the “conservative envelope”. Both, the default and conservative curves, are shown in Fig. 3.

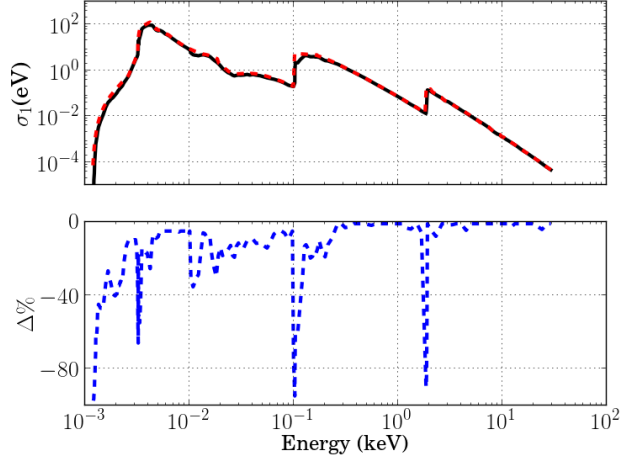

Figure 3: Top Panel: Real part of the complex conductivity  $\sigma_1 = \text{Re}(\tilde{\sigma})$  for Si. The red-dashed curve is  $\sigma_1$  from Ref [3]. The black-solid curve is the conservative  $\sigma_1$  curve determined by applying the reduction in the cross section to the baseline due to measurement uncertainties and temperature and electric field effects. Bottom Panel: Percent difference between the conservative  $\sigma_1$  and  $\sigma_1$  from Ref [3].

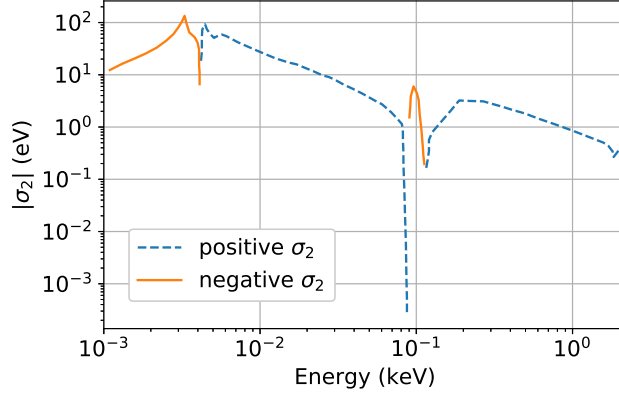

Figure 4: Imaginary part of the complex conductivity  $\sigma_2 = \text{Im}(\tilde{\sigma})$  for Si. The blue-dashed (orange-solid) curve are positive (negative) values of  $\sigma_2$  from Ref [3].

### 1.2.2 Imaginary Part of the Complex Conductivity: Phase Lag of the System

The imaginary value of the conductivity,  $\sigma_2$ , can be interpreted as the delay of the charge carrier response to quick changes in the electric field. This value depends on the energy of the incoming photon, or in the context of dark photon searches, on the energy of the incoming dark photon. In case of  $\sigma_2$ , hardly any literature exists that would have allowed a similarly detailed study as for  $\sigma_1$ . For this reason, only one set of  $\sigma_2$  values was used for the limit calculation. These values are from Ref [3] and are included in this data release in the following file:

- `Conductivity_Si_keV_eV_Imaginary.tsv`.

The photon energy scale is again in keV, the  $\sigma_2$  scale is in eV. The absolute values of  $\sigma_2$  are shown in Fig. 4.

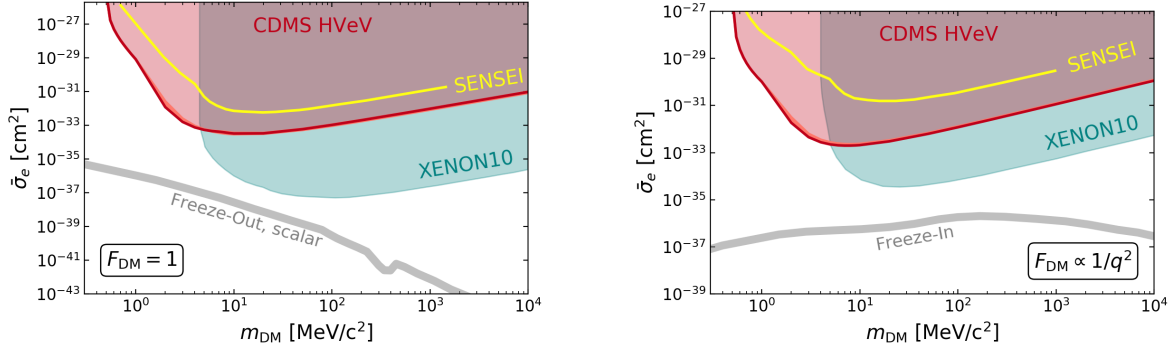

(a) HVeV limit on the DM-electron scattering cross section  $\bar{\sigma}_e$  for DM interacting with electrons via a heavy dark photon ( $F_{\text{DM}} = 1$ ) compared to the XENON10 and SENSEI results as well as the freeze-out target [4, 5, 6].

(b) HVeV limit on the DM-electron scattering cross section  $\bar{\sigma}_e$  for DM interacting with electrons via an ultra-light dark photon ( $F_{\text{DM}} \propto q^2$ ) compared to the XENON10 and SENSEI results as well as the freeze-in target [4, 5, 6].

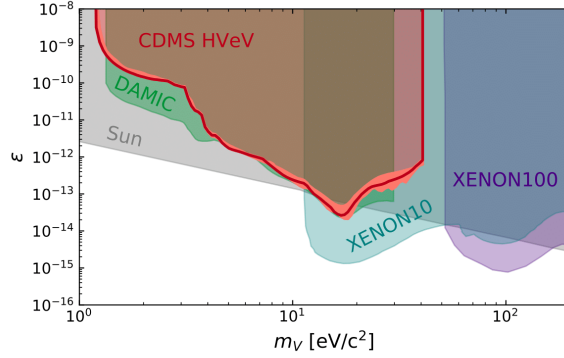

(c) HVeV limit (red line) on dark photon kinetic mixing  $\varepsilon$  compared to the results from DAMIC, XENON10 and XENON100 [[7], and references therein.]

Figure 5: HVeV DM search limits as published in Ref [1]. The red line is the nominal HVeV limit with a Fano factor of 0.155. The salmon-colored region indicates the systematic uncertainties due to varying the Fano factor in the ionization model between the lowest mathematically possible value and 1, as well as due to uncertainties in the photoelectric cross section for dark photon absorption.

### 1.3 Exclusion limits

The files containing the three published Ref [1] exclusion limits, including their bands, are described in this section. The respective limits are shown in Fig. 5. For each limit, one file is included in this data release:

- HVeV-Run1-DMe-F1-Limit.tsv (Fig. 5a),
- HVeV-Run1-DMe-Fq2-Limit.tsv (Fig. 5b),
- HVeV-Run1-DarkPhoton-Limit.tsv (Fig. 5c).

The first two files contain the scattering cross section limit on DM scattering off electrons for two different DM form factors:  $F_{\text{DM}} = 1$  and  $F_{\text{DM}} \propto q^{-2}$ , where  $q$  is the momentum transfer. The form factor is indicated in the file name as “F1” and “Fq2”, respectively. The third file contains the limit on dark photon kinetic mixing. All files consist of four columns:

- Column 0: DM mass in  $\text{MeV}/c^2$  for DM-e scattering and in  $\text{keV}/c^2$  for dark photon absorption.

- Column 1: nominal limit.
- Column 2: upper bound of limit band.
- Column 3: lower bound of limit band.

The limit bands represent the maximum systematic uncertainty induced by an uncertainty on the Fano factor (see Sec. 2) and, in the case of dark photon absorption, on the photoelectric cross section (see Sec. 1.2.1).

## 2 Detector Response Model

To compute the detector response to a given modeled input, recoil energy needs to be converted to number of  $e^-h^+$  pairs,  $n_{\text{eh}}$ . The mean number of  $e^-h^+$  pairs produced by an electron recoil of energy  $E_\gamma$  is given by the piece-wise function

$$\langle n_{\text{eh}}(E_\gamma) \rangle = \begin{cases} 0 & E_\gamma < \epsilon_{\text{gap}} \\ 1 & \epsilon_{\text{gap}} < E_\gamma < \epsilon_{\text{eh}} \\ E_\gamma/\epsilon_{\text{eh}} & \epsilon_{\text{eh}} < E_\gamma \end{cases} \quad (1)$$

where  $\epsilon_{\text{gap}} = 1.12$  eV and  $\epsilon_{\text{eh}} = 3.8$  eV [8]. The detector resolution for the Run 1 data was  $\sigma_{\text{eh}} = 0.09$   $e^-h^+$  pairs [1]. The probability distributions in the first two cases are delta functions, necessary in order to conserve energy. In the third case, discrete distributions are generated with an arbitrary Fano factor,  $F$ , defined as

$$F = \frac{\sigma^2}{\mu} \quad (2)$$

where  $\mu = \langle n_{\text{eh}} \rangle$  is the mean of the distribution, and  $\sigma^2$  is the variance. A completely uncorrelated (Poisson) process has a Fano factor of 1, but in most radiation detectors Fano factors on the order of 0.1-0.2 are found due to the fact that large deviations from the mean are kinematically suppressed.

Probability distributions for a given mean and Fano factor were generated using a binomial distribution with  $n$  trials of probability  $p$ . The binomial distribution has variance  $\sigma^2$  and mean  $\mu$  that obey the relations

$$\mu = np \quad (3)$$

$$\sigma^2 = np(1-p) = \mu(1-p) \quad (4)$$

This allows to calculate the  $n$  and  $p$  values from the Fano factor and mean number of  $e^-h^+$  pairs as

$$F = \frac{\sigma^2}{\mu} = (1-p) \rightarrow p = 1-F \quad (5)$$

$$n = \frac{\mu}{p} = \frac{\mu}{1-F} \quad (6)$$

The caveat to these equations is that the binomial distribution is quantized, and thus  $n$  is an integer; this means that we have to interpolate between the distributions for the integers directly above and below the fractional mean value given by the mean and Fano factor combination. This is done according to the following

procedure:

$$n_l(\mu, F) = \text{floor} \left( \frac{\mu}{1 - F} \right) \quad (7)$$

$$n_h(\mu, F) = \text{ceil} \left( \frac{\mu}{1 - F} \right) \quad (8)$$

$$F_l(\mu, F) = \mu/n_l(\mu, F) \quad (9)$$

$$F_h(\mu, F) = \mu/n_h(\mu, F) \quad (10)$$

$$\Delta F(\mu, F) = \frac{F - F_l(\mu, F)}{F_h(\mu, F) - F_l(\mu, F)} \quad (11)$$

$$P_l(x|\mu, F) = \text{Binomial}(x|n_l(\mu, F), 1 - F_l(\mu, F)) \quad (12)$$

$$P_h(x|\mu, F) = \text{Binomial}(x|n_h(\mu, F), 1 - F_h(\mu, F)) \quad (13)$$

$$P(x|\mu, F) = P_l(x|\mu, F)(1 - \Delta F(\mu, F)) + P_h(x|\mu, F)\Delta F(\mu, F) \quad (14)$$

where  $P(x|\mu, F)$  is the final probability distribution. This is the weighted mean of two binomial distributions given a non-integer mean, with weights defined by how close the Fano factor of the binomial distribution is to the intended Fano factor. One can verify that this weighting gives the correct mean and Fano factor.

For the limit in Ref [1], the measured high energy value  $F = 0.155$  was used. However each limit was also calculated with the lowest mathematically possible value of  $F$ , and  $F = 1$ .

### 3 Limit Calculation

In order to compute DM search limits, three main inputs are needed: the experimental spectrum, the DM model to be probed, and a limit setting technique. This section will describe each of these pieces, which together resulted in the published HVeV Run 1 DM search limits shown in Sec. 1.3.

#### 3.1 Experimental Input

The HVeV Run 1 experimental inputs are the observed energy spectrum (Fig. 1, Sec. 1.1.1), the signal efficiency (Fig. 2c, Sec. 1.1.2), the analysis thresholds (both an upper and lower limit), and the total exposure. The lower analysis threshold is  $0.7 e^-h^+$  pairs, and the upper threshold is  $10 e^-h^+$  pairs. The total exposure after all livetime cuts were applied was 0.488 g-days. No further experimental information related to the HVeV detector is necessary to calculate limits for the DM models presented in Ref [1].

#### 3.2 Dark Matter Models

Three DM models were probed in Ref [1]: light DM interacting with electrons via a heavy dark photon, light DM interacting with electrons via an ultra-light dark photon, and dark photons kinetically mixing with the Standard Model (SM) and being a relic DM candidate themselves. The first two models and their event rate calculations are outlined in Sec. 3.2.1. The third model and its event rate calculation is outlined in Sec. 3.2.2.

##### 3.2.1 Light DM - Electron Scattering

The scattering rate of DM against electrons is given by the equation

$$\frac{dR}{d \ln E_R} = V_{\text{det}} \frac{\rho_{\text{DM}}}{m_{\text{DM}}} \frac{\rho_{\text{Si}}}{2m_{\text{Si}}} \bar{\sigma}_e \alpha \frac{m_e^2}{\mu_{\text{DM},e}^2} I_{\text{crystal}}(E_e; F_{\text{DM}}), \quad (15)$$

where  $V_{\text{det}} = 1 \times 1 \times 0.4 \text{ cm}^3$  is the detector volume,  $\rho_{\text{DM}}$  is the relic DM density (assuming  $\rho_{\text{DM}} \approx 0.3 \text{ GeV/cm}^3$ ),  $m_{\text{DM}}$  is the DM mass,  $\rho_{\text{Si}} = 2.33 \text{ g/cm}^3$  and  $m_{\text{Si}} = 28.09 \text{ amu}$  are the silicon density and mass,  $\bar{\sigma}_e$  is the DM-e scattering cross section,  $\mu_{\text{DM},e}$  is the reduced mass of the DM electron system,  $I_{\text{crystal}}$  is the crystal form factor,  $E_e$  is the electron energy and  $F_{\text{DM}}$  is the DM form factor.

Two common benchmark models were used to calculate the limits shown in Figs. 5a and 5b. The first is a model with no form factor,  $F_{\text{DM}} = 1$ , assuming DM interacts with electrons via a heavy dark photon. The second is a model with  $F_{\text{DM}} = \alpha^2 m_e^2 / q^2$ , assuming DM interacts with electrons via an ultra-light dark photon.

The rate calculation Eq. 15 is further dependent on  $I_{\text{crystal}}$ , and thus requires knowledge of the electronic structure of the target crystal. The rate calculation including the integration of  $I_{\text{crystal}}$  is provided by the QEdark tool. Information on the QEdark calculation as well as the calculated rates for silicon are publicly available at <http://ddldm.physics.sunysb.edu/ddldm/>. The published calculations describe the yield for electron recoils up to 50 eV, both as continuous (in units of deposited energy) and as quantized (in  $e^-h^+$  pairs) differential rates. For Ref [1], the continuous rates were used, quantized using our own, more sophisticated quantization model (described in Sec. 2), and convolved with the  $e^-h^+$  pair energy resolution  $\sigma_{\text{eh}}$  of the HVeV detector.

### 3.2.2 Dark Photon Absorption

The probed dark photon model assumes kinetic mixing between the dark photon and the SM photon. The predicted event rate for dark photon absorption is given by

$$R = V_{\text{det}} \frac{\rho_{\text{DM}}}{m_V} \varepsilon_{\text{eff}}^2 (m_V, \tilde{\sigma}) \sigma_1(m_V), \quad (16)$$

where  $m_V$  is the dark photon mass and  $\varepsilon_{\text{eff}}$  is an effective mixing angle.  $\varepsilon_{\text{eff}}$  is directly related to the parameter of interest, the kinetic mixing parameter  $\varepsilon$ :

$$\varepsilon_{\text{eff}}^2 = \varepsilon^2 \cdot \frac{m_V^4}{[m_V^2 - \text{Re}\Pi]^2 + [\text{Im}\Pi]^2}. \quad (17)$$

$\Pi$  is the polarization tensor,

$$\Pi(E = m_V c^2) \approx -i \cdot \tilde{\sigma} \cdot m_V c^2, \quad (18)$$

which can be substantially altered by in-medium effects. For  $m_V \gtrsim 100 \text{ eV}/c^2$   $\varepsilon$  is well-approximated by  $\varepsilon_{\text{eff}}$ . For smaller dark photon masses, as in [1], in-medium corrections can no longer be neglected, and Eq. 17 has to be used. Both Eq. 16 and Eq. 17 require knowledge of  $\sigma_1 = \text{Re}(\tilde{\sigma})$ , the photoelectric cross section (see Fig. 3). Equation 17 further requires knowledge of  $\sigma_2 = \text{Im}(\tilde{\sigma})$  (see Fig. 4).

The dark photon spectrum resulting from Eq. 16 in the continuous regime consists of a sharp line at the electron recoil energy corresponding to the dark photon mass, broadened by the energy resolution of the detector. To calculate the dark photon signal spectrum in the quantized regime, the ionization model described in Sec. 2 was employed, and the quantized spectrum was again convolved with  $\sigma_{\text{eh}}$ . Since the expected dark photon signal spectrum is based on Eq. 16 it is related to  $\varepsilon_{\text{eff}}$ . Thus also the resulting limit is initially set on  $\varepsilon_{\text{eff}}$ . The in-medium correction Eq. 17 is applied on the  $\varepsilon_{\text{eff}}$  limit only afterwards, converting it into a  $\varepsilon$  limit, the limit of interest.

### 3.3 Limit Setting

The 90% confidence level upper limit calculation is based on the high-statistics Optimum Interval (OI) method [2]. This method was applied without background subtraction. For a non-zero background level, the limit is stronger when the DM signal expectation is larger than the background level within the identified optimum interval. It is thus beneficial to remove regions from the data that cannot possibly include a significant amount of DM events. The HVeV data spectrum is continuous (see Fig. 1) while the expected DM signal is quantized. As a result, virtually no DM signal is expected between the quantization peaks and those regions can be safely excluded from the ROI. To be more precise, events further than  $2\sigma_{\text{eh}}$  away from the Gaussian  $e^-h^+$  peaks' mean were removed by using the efficiency curve shown in Fig. 2c. In doing so, an ROI is generated that contains, by definition, 95% of the expected DM signal. This ROI was used for all three published limits including their bands shown in Fig. 5.

Having selected the ROI for the limit calculation, the next parameters of interest are the Fano factor  $F$  and, in the case of dark photon absorption, the photoelectric cross section  $\sigma_1$ . To obtain the three nominal

limits, a Fano factor  $F = 0.155$  was used for all three calculations, and the “reference data” for  $\sigma_1$  (see Sec. 1.2.1) was used for the dark photon kinetic mixing limit. To obtain the limit bands, the calculation was repeated, once with the lowest mathematically possible value of  $F$  and once with  $F = 1$ . The dark photon limit calculation was further repeated with the “conservative data” for  $\sigma_1$  (see Sec. 1.2.1) and also corrected for in-medium effects using this “conservative data” in Eq. 17. The bands shown in Fig. 5 represent the envelope of the resulting limits.

### 3.3.1 Optimum Interval Software

The core OI software is publicly available from the link in Ref [9], including documentation for individual scripts. These files were previously adapted to use double-precision variables, as opposed to single-precision variables. The double-precision versions of these files were released by the SuperCDMS Collaboration as part of the CDMSlite Run2 data release [10]. For the published HVeV dark photon limit calculation, it was necessary to increase the precision of probed DM masses, as the HVeV detector covers dark photon masses as low as about  $1 \text{ eV}/c^2$ , as opposed to typical WIMP masses at the  $\text{GeV}/c^2$  scale. For convenience, all files (except the example files) from Ref [9] are provided in the `OI_code` directory of this release with these precision improvements implemented. The OI code is written in FORTRAN, with the primary function contained in `CalcOptLim3.f`. The code was compiled for a Unix operating system, which produced the `CalcOptLim3` executable. It can be recompiled on any Unix system by running the command

```
gfortran -frecord-marker=4 -o CalcOptLim3 CalcOptLim3.f UpperLimNew3.f y_vs_CLf2.f
CMaxinfNew2.f ConfLev2.f ConfLevNew2.f Cinf2.f CERN.Stuff2.f
```

or

```
f77 -o CalcOptLim3 CalcOptLim3.f UpperLimNew3.f y_vs_CLf2.f CMaxinfNew2.f ConfLev2.f
ConfLevNew2.f Cinf2.f CERN.Stuff2.f
```

The function in `CalcOptLim3.f` uses an input file (`ULinput`) and an output file (`ULoutput`). The expected format of the `ULinput` file is documented in `CalcOptLim3.f` and requires the list of events in the data set of interest. The input values contained in the input file depend on the model assumptions, and thus on the probed DM model, and on any further model assumptions (such as the ionization model and the photoelectric cross section assumptions employed in this result). The `ULoutput` file is generated automatically and contains the resulting limit information. In the case of DM searches this is typically the coupling strength (or a correction factor on a fixed coupling strength) as a function of the DM mass. Details on the `ULoutput` content and format are also found in `CalcOptLim3.f`.

## References

- [1] SuperCDMS Collaboration. First Dark Matter Constraints from a SuperCDMS Single-Charge Sensitive Detector. *Phys. Rev. Lett.*, 121(5):051301, 2018. doi: 10.1103/PhysRevLett.122.069901,10.1103/PhysRevLett.121.051301. [Erratum: *Phys. Rev. Lett.*122,no.6,069901(2019)].
- [2] S. Yellin. Extending the optimum interval method. *ArXiv e-prints*, September 2017. URL <https://arxiv.org/abs/0709.2701>.
- [3] Y. Hochberg, T. Lin, and K. M. Zurek. Absorption of light dark matter in semiconductors. *Phys. Rev. D*, 95(2):023013, January 2017. doi: 10.1103/PhysRevD.95.023013.
- [4] Rouven Essig, Aaron Manalaysay, Jeremy Mardon, Peter Sorensen, and Tomer Volansky. First Direct Detection Limits on sub-GeV Dark Matter from XENON10. *Phys. Rev. Lett.*, 109:021301, 2012. doi: 10.1103/PhysRevLett.109.021301.
- [5] M. Crisler et al. SENSEI: First Direct-Detection Constraints on sub-GeV Dark Matter from a Surface Run. *Phys. Rev. Lett.*, 121(6):061803, 2018. doi: 10.1103/PhysRevLett.121.061803.

- [6] M. Battaglieri et al. S Cosmic Visions: New Ideas in Dark Matter 2017: Community Report. *ArXiv e-prints*, July 2017. URL <http://arxiv.org/abs/1707.04591>.
- [7] A. Aguilar-Arevalo et al. First Direct-Detection Constraints on eV-Scale Hidden-Photon Dark Matter with DAMIC at SNOLAB. *Phys. Rev. Lett.*, 118(14):141803, 2017. doi: 10.1103/PhysRevLett.118.141803.
- [8] V S Vavilov. Radiation ionization processes in germanium and silicon crystals. *Soviet Physics Uspekhi*, 4(5):761, 1962. URL <http://stacks.iop.org/0038-5670/4/i=5/a=A12>.
- [9] Steven Yellin. *Software for computing an upper limit given unknown background*, 2011 (last accessed September 20, 2018). URL <http://titus.stanford.edu/Upperlimit/>.
- [10] SuperCDMS. *Public Release #1 of CDMsLite Run 2 Data*, 2017 (last accessed September 20, 2018). URL [http://cdms.berkeley.edu/data\\_releases.html](http://cdms.berkeley.edu/data_releases.html).
