# Supplementary material for: First Dark Matter Constraints from a SuperCDMS Single-Charge Sensitive Detector
Source: arXiv:1804.10697 ancillary file (2020-12-23)
Supplement: Supplementary file 2 [file PE_XSec_Supplement_V2-3.pdf]

# Supplemental Material: First Dark Matter Constraints from SuperCDMS Single-Charge Sensitive Detectors

The dark photon model used in this work is described in Ref. [1]. This model assumes an interaction between the dark photon and normal matter using the standard model photon as a mediator. The interaction rate is dependent on the photoelectric cross section, $\sigma_{p.e.}$, through the real part of the complex conductivity, $\sigma_1$.

The photoelectric cross section is material specific and an energy-dependent quantity for which there are tabulated measured values available. A literature search was performed for silicon (Si) $\sigma_{p.e.}$ measurements spanning the optical to x-ray energy range ($\sim$ 1 eV – 30 keV). Particular emphasis was placed on finding data in the low-energy (< 10 eV) and low temperature (< 100 K) regimes. Table I lists the sources from this literature review that were used in this analysis. There are only a few available $\sigma_{p.e.}$ measurements below 100 K, none of which covered the full energy range between 1 and 10 eV. Additionally, these measurements were carried out without an external electric field applied to the samples. Thus, the available data from the literature search do not properly reflect the operating conditions of the SuperCDMS detector in this work. Therefore, $\sigma_{p.e.}$ had to be analytically estimated taking into consideration the effects of a low operating temperature (33–36 mK) and an applied electric field. For this analysis the smallest Si $\sigma_{p.e.}$ measured at each energy is used as a baseline value. This baseline represents an upper limit to the dark photon normal matter interaction before the effects of temperature and electric field are considered.

| Ref. | Energy Range | Temp. (K) |
|---|---|---|
| [2] | 10 eV – 30 keV | Not Specified |
| [3] | 1 eV – 2 keV | Not Specified |
| [4] | 1–5 eV | 300 |
| [5] | 1–1.3 eV | 415–4.2 |
| [6] | 1–3.5 eV | 300–77 |
| [7] | 1–5 eV | 300–77 |
| [8] | 10–90 eV | Not Specified |
| [9] | 30–120 eV | Not Specified |
| [10] | 90–210 eV | 300 |
| [11] | 6–20 keV | 77 |

TABLE I. References for the photoelectric cross section of Si. The values were used to determine a conservative value for $\sigma_1$ in the analysis. The temperature (where specified) and energy ranges for each source are indicated.

## Dependence on Temperature

Temperature dependence is expected to be significant where indirect absorption (phonon-mediated transitions to the conduction band) is the dominant process, as it is directly dependent on the number density of thermal phonons. Only indirect absorption is allowed by momentum conservation below the direct band gap, in the energy range 1.12–3.2 eV. Within this energy region, the baseline $\sigma_{p.e.}$ contains measurements made at 4.2 and 77 K. The indirect absorption coefficient is proportional to (see Ref. [12]),

$$\alpha_{\text{ind}}(T) \propto \frac{(E - E_g + E_q)^2}{e^{E_q/k_B T} - 1} + \frac{(E - E_g - E_q)^2}{1 - e^{-E_q/k_B T}}, \qquad (1)$$

where $E$ is the photon energy, $E_g$ is the indirect band gap energy, and $E_q$ is the phonon energy. The first term on the RHS of Eq. 1 is the phonon absorption process, while the second term is the phonon emission process. The variation in $\sigma_{p.e.}$ was determined using Eq. 1 when changing the temperature from 77 K to 30 mK; there is no significant change between 4.2 K and 30 mK. The reduction of $\sigma_{p.e.}$ for the indirect absorption at 30 mK relative to the measured value at 77 K is shown by the green curve in Figure 1.

Direct absorption depends indirectly on temperature through variation in the direct band gap energy. Lowering the temperature from 300 K to 30 mK increases the direct band gap by $\sim$2%. We estimated the variation in $\sigma_{p.e.}$ by shifting the data from Ref. [3] by 2% and calculating the resulting change in cross section. This was done between 3.2 and 4.3 eV to account for the different direct transitions [13], and is shown by the red curve in Figure 1.

## Dependence on Applied Electric Field

The change in direct absorption due to an applied electric field (the Franz-Keldysh effect) was calculated using Eq. (4) in Ref. [14]:

$$\begin{aligned}\Delta\alpha(\omega, F) = \frac{C}{\omega}\Bigg\{ & \theta_F^{1/2}\left[\left|\frac{d\text{Ai}(\beta)}{d\beta}\right|^2 - \beta\,|\text{Ai}(\beta)|^2\right] \\ & - 0.3187(\omega - \omega_1)^{1/2}\Bigg\}, (\omega > \omega_1) \qquad (2) \\ = \frac{C}{\omega}\theta_F^{1/2} & \left[\left|\frac{d\text{Ai}(\beta)}{d\beta}\right|^2 - \beta\,|\text{Ai}(\beta)|^2\right], (\omega < \omega_1)\end{aligned}$$

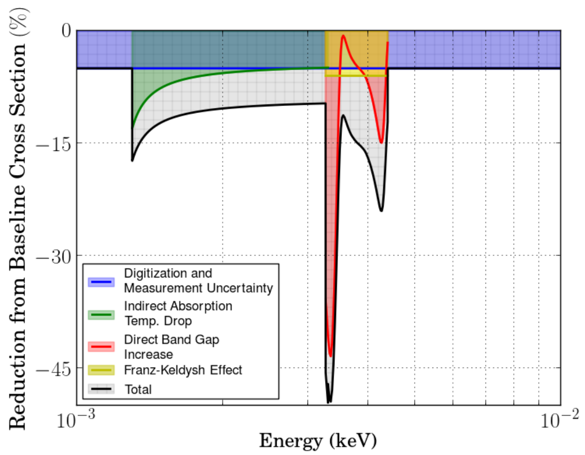


FIG. 1. Reduction in cross section from the baseline for Si between 1 and 10 eV. The reduction due to temperature dependence in the indirect absorption was determined by calculating the percentage change in cross section from 77 K to 30 mK. Corrections due to electric field assumed a field strength of 400 V/cm. The total reduction was calculated by consecutively multiplying the individual reductions.

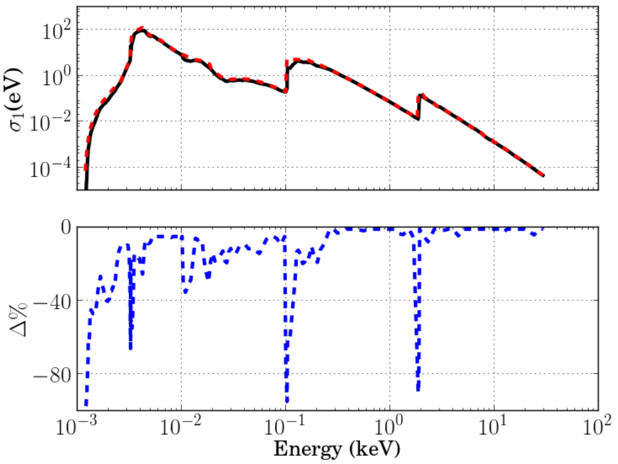


FIG. 2. Top Panel: $\sigma_1$ curves for Si. The red-dashed curve is $\sigma_1$ from Ref. [1]. The black-solid curve is the conservative $\sigma_1$ curve determined by applying the reduction in the cross section shown in Figure 1 to the baseline $\sigma_{p.e.}$. Bottom Panel: Percent difference between the conservative $\sigma_1$ and $\sigma_1$ from Ref. [1].

where $\omega$ is the photon energy, $F$ is the field strength, $\mathrm{Ai}(\beta)$ is the Airy Function[1], and $\beta = (\omega_1 - \omega)/\theta_F$. The parameters $C = 2.5 \cdot 10^{14}$ cm$^{-1}$ sec$^{-1/2}$ and $\omega_1 = 4.86 \cdot 10^{15}$ sec$^{-1}$ are the scaling constant and direct band gap energy for Si, respectively, and $\theta_F^3 = (e^2F^2/2\mu\hbar)$, where $\mu$ is the reduced mass of the electron-hole pair. The calculations showed significant changes only at the direct absorption threshold. We estimated the variation of the $\sigma_{p.e.}$ by calculating the change in $\sigma_{p.e.}$ after applying the effect of an electric field to the data from Ref. [3]. A variation of $\sim 6\%$ was observed for a maximum field strengths of 400 V/cm corresponding to the applied electric field used in this paper. The variation in $\sigma_{p.e.}$ due to this effect is shown by the yellow curve in Figure 1.

[1] Ref. [14] uses a slightly different convention for the normalization of the Airy Function than assumed in Eq. 2 above. A multiplicative factor of $\pi$ has therefore been inserted when using their result to account for this difference in normalization.

### Uncertainty in Measured $\sigma_{p.e.}$

At high energies, above 230 eV, the spread in the measured $\sigma_{p.e.}$ from reference to reference is small. At low energies the spread tends to be larger. In order to account for this variation of the measurements found in the literature, an uncertainty of 5% below 230 eV is shown in blue in Figure 1. This flat reduction also accounts for small errors due to digitization of the data and variation due to material density changes.

Changes in $\sigma_{p.e.}$ due to diminishing free carrier absorption were considered but determined to be negligible due to the extremely low free carrier density in the crystals, even at room temperature.

### Conservative Values for $\sigma_1$

The top panel in Figure 2 shows the conservative $\sigma_1$ curve for Si resulting from this analysis. Conservative refers to the smallest $\sigma_1$ values that result in the largest dark photon mixing parameter values. This curve was determined by applying the reduction in the $\sigma_{p.e.}$ shown in Figure 1 to the baseline $\sigma_{p.e.}$. Also shown is the $\sigma_1$ curve from Ref. [1]. The bottom panel in Figure 2 shows the percent difference between the two $\sigma_1$ curves. This discussion focused on the photoelectric cross section. For the index of refraction, which also impacts the interaction rate, we use the same model as Ref. [1].

[1] Y. Hochberg, T. Lin, and K. M. Zurek, Phys. Rev. D **95**, 023013 (2017), arXiv:1608.01994 [hep-ph].
[2] B. Henke, E. Gullikson, and J. Davis, Atomic Data and Nuclear Data Tables **54**, 181 (1993).
[3] D. F. Edwards, in *Handbook of Optical Constants of Solids*, edited by E. D. Palik (Academic Press, Burlington, 1997) pp. 547 – 569.
[4] M. A. Green and M. J. Keevers, Progress in Photovoltaics: Research and Applications **3**, 189 (1995).
[5] G. G. Macfarlane, T. P. McLean, J. E. Quarrington, and V. Roberts, Phys. Rev. **111**, 1245 (1958).
[6] W. C. Dash and R. Newman, Phys. Rev. **99**, 1151 (1955).

[7] S. E. Holland, D. E. Groom, N. P. Palaio, R. J. Stover, and M. Wei, IEEE Transactions on Electron Devices **50**, 225 (2003).
[8] B. L. Henke, J. C. Davis, E. M. Gullikson, and R. C. C. Perera, Report Number: LBL-26259, Berkeley (1988).
[9] E. M. Gullikson, P. Denham, S. Mrowka, and J. H. Underwood, Phys. Rev. B **49**, 16283 (1994).
[10] C. Gähwiller and F. C. Brown, Phys. Rev. B **2**, 1918 (1970).
[11] R. Nathuram, I. S. Sundara Rao, and M. K. Mehta, Phys. Rev. A **37**, 4978 (1988).
[12] J. I. Pankove, *Optical Processes in Semiconductors* (Englewood Cliffs, N.J.: Prentice-Hall, 1971).
[13] N. Ashcroft and N. Mermin, *Solid State Physics*, HRW international editions (Holt, Rinehart and Winston, 1976).
[14] B. O. Seraphin and N. Bottka, Phys. Rev. **139**, A560 (1965).
